# Supplementary material for: Lion Secretly Solves Constrained Optimization: As Lyapunov Predicts
Source: arXiv:2310.05898 source file (2025-07-01)
Supplement: Supplementary file 1 [file appendix.tex]

\subsection{Experiments and Details}\label{sec:exps}
Confirming that :ion is a (near) optimal within the design space, but there are opportunities left. In this section, we show possible ways to extend Lion and explore perspective optimization schemes within our framework. 


By taking a weighted combination of the Hamiltonian and Mirror Descent Components, we get 
\bb 
x_{t+1} & = x_t  - \gamma \left [ u  \dd\phi(m_t + \beta \dd f(x_t)) + (1- u)\dd \phi(m_t) \right ] \\ 
 m_{t+1}&  =  m_t + \beta (\dd f(x_t) - \red{u} m_t),
\ee 
where $u$ can be any positive number. If $u>1$, it corresponds to extrapolating the direction towards the $\phi(m_t + \beta \dd f(x_t)) - \dd \phi(m_t)$ direction.





\subsection{Non-differentiable $\phi$ in Continuouus Time}
\label{sec:non-diff}

\red{maybe state the non-differentiable framework in the beginning}

%\qq{discuss the non-differentiblity here}
We show that, intriguingly, 
$\beta>0$ plays a crucial role here. 
The case when $\beta=0$ does not  have the monotonic descending property. 
%\todo{illustrate the example of L1 and L2 here.}

We start with introducing some basic facts. A convex function $\phi$  on $\RR^d$ is differentiable except on countable many points. 
On the non-differentiable points, the behavior of $\phi$ is characterized by its sub-differential, denoted by $\partial \phi(x)$, which is the  set of vectors $d\in \partial \phi(x)$ satisfying  
\bbb  \label{equ:phi}
\phi (y) \geq \phi (x) + d \tt (y-x), ~~\forall y. 
\eee  
The sub-differential is always non-empty. if $x$ is differentiable point of $x$, then $\partial \phi(x)$ includes a single element, which is the derivative $\dd \phi(x)$ in the classical sense. 

Exchanging the order of $x$ and $y$ in \eqref{equ:phi}, we have, for $b \in \partial \phi(y)$, 
\bb
\phi(x) \geq \phi(y) - b \tt (y-x).
\ee 

Summing the two equations gives 
$$
D_\phi(x, y) 
\defeq 
\inf_{d_x\in\partial \phi(x), d_y\in \partial \phi(y)} (d_x - d_y)\tt (x-y) \geq 0.
$$
A point $x^*$ is a minimum of $\phi$ iff $0 \in \partial \phi(x^*)$. Hence, 
if $0$ is the unique minimum of $\phi$, then $D_\phi(x, 0) =0$ iff $x=0$. 

\begin{exa}
For $\phi(x) = \norm{x}_1 = \sum_{i=1}^d \abs{x_i}$, we have 
$\partial \phi(x) =  \partial_{1} \phi(x) \times \cdots \times \partial_d \phi(x)$  with 
\bb \partial_i \phi(x) = 
\begin{cases} 
\{\sign(x_i)\} & \text{if $x_i \neq 0$} \\
[-1,1] & \text{if $x_i=0$}
\end{cases} 
 \ee 
where $\times $ denotes the Cartesian product of sets. 
%we have 
\bb 
D_\phi(x, y) 
& =  
\begin{cases}  
(\sign(x) - \sign(y)) \tt (x-y)  & \text{if $xy\neq 0$}  \\
0 & \text{if xy =0} 
\end{cases}
& =  \begin{cases}
2 \abs{x-y} & \text{if $xy < 0$} \\
0 & \text{if $xy\geq0$}. 
\end{cases}
\ee 
\end{exa}

Another important property of $\partial f(x)$ that we will use is 
$$
\sup_{d \in \partial \phi(x)} \{ d\tt u \} 
= \phi_+'(x; u)\defeq  \lim_{\epsilon \to 0^+} 
\frac{\phi(x+ \epsilon u) - \phi(x)}{\epsilon}, 
$$
where $\phi_+'(x,u)$ is called the 
 right directional derivative of $\phi$ in the direction of $u$. 
One can show that $\phi_+'(x,u)$ always exists at every point $x$ and direction $u$. 


%Then it is easy to show from\eqref{equ:phi} that $$D_{\dd\phi}(x, y)\defeq (\dd \phi(x) - \dd \phi(y))\tt (x - y) \geq 0. $$

%Define the as $$\phi'_+(x; d) = \lim_{\epsilon \to 0^+} \frac{\phi(x+ \epsilon d) - \phi(x)}{\epsilon}. $$
%Then we have 


\begin{thm}
Assume $\phi$ is convex on $\RR^d$ 
\red{with $0$ as a minimum point},
%whose% unique minimum is $x=0$,  
and $\dd \phi(x)$ is a subgradient of $\phi$ in that  $\dd \phi(x) \in \partial \phi(x)$ for every $x$. 
Assume $\red{\alpha, \beta} >0$. 
Assume $f$ 
 is differentiable. 
%and $\phi$ is convex with $\vv  0$ as 
its minimum point.  
%with $\dd\phi(\vv 0)=\vv 0$. 
Then following \eqref{equ:lionode}, 
the Hamiltonian $H(\vv x,\vv m)$ decreases monotonically in that 
%in is reviewed a%
$$
\ddtp  H(\vv x_t, \vv m_t)
%=  \lim_{\epsilon \to 0^+} \frac{1}{\epsilon}(H(\vv x_{t+\epsilon}, \vv m_{t+\epsilon})) - H(\vv x_t, \vv m_t)
= - \Delta(x_t, m_t) \leq 0, 
$$ 
with 
$$
 \Delta(x_t, m_t) = \frac{1}{\beta} D_\phi(\vv m_t+\beta \dd f(\vv x_t), \vv m_t) 
+ \eta D_\phi(\vv m_t, \vv 0)
$$
where $\ddtp$ denote the right derivative w.r.t. time, that is  
$\ddtp  H_t \defeq 
 \lim_{\epsilon \to 0^+} \frac{1}{\epsilon}(H_{t+\epsilon} - H_t)$ with  $H_t =H(\vv x_{t+\epsilon}, \vv m_{t+\epsilon}))$. 
 
Moreover, 
\red{if $\vv 0$ is the unique minimum of $\phi$}.  
if $\phi$ is strictly convex, 
the system must converge to a stationary point of $H(\vv x,\vv m)$
on which we have $\vv m =0 $ and $\dd f(\vv x) =0$. 
\end{thm} 
\begin{proof}
\bb 
\ddtp H(\vv x_t, \vv m_t) 
& = 
\ddtp f(x_t) + \ddtp \phi(m_t).
%\lim_{\epsilon \to 0^+} 
%\dd_{\vv x} 
%\frac{1}{\epsilon} H(\vv x_{t+\epsilon}, m_{t+\epsilon}) - H(\vv x_{t}, \vv m_{t+\epsilon} )  
%+ \lim_{\epsilon  \to 0^+ } H(\vv x_t, \vv m_{t+\epsilon}) -
%H(\vv x_t, \vv m_{t})  \\ 
\ee
Due to the differentiability of $f$, we have $\ddtp f(x_t) = \dd f(x_t) \tt \dot x_t$. It mains to handle the $ \ddtp \phi(m_t)$ part. 

\bb 
\ddtp \phi(m_t) %H(\vv x_t, \vv m_t) 
%& = \dd_{\vv x} H(\vv x_t, m_t) \tt \dot{\vv x}_t + \lim_{\epsilon  \to 0^+ } H(\vv x_t, \vv m_{t+\epsilon}) -
%H(\vv x_t, \vv m_{t})  \\ 
 & = \lim_{\epsilon\to 0^+}\frac{\phi(m_{t+\epsilon}) - \phi(m_t)}{\epsilon}\\   
 %+ \lim_{\epsilon\to 0^+} \frac{\phi(m_{t+\epsilon}) - \phi(m_t + \epsilon \dot m_t)}{\epsilon}  \\
 & = \lim_{\epsilon\to 0^+}\frac{\phi(m_{t}+\epsilon \dot m_t) - \phi(m_t)}{\epsilon}  \ant{$m_{t+\epsilon}\to m_{t}+\epsilon \dot m_t$ and all convex functions are continuous} \\
 & = \sup_{d\in \partial \phi(m_t)} 
 d \tt \dot m_t \\
 & = \sup_{d \in \partial \phi(m_t)} 
 d \tt \dot m_t.
\ee 
%Hence, 
Write $\tilde m_t = m_t + \beta \dd f(x_t)$. We have 
\bb 
\ddtp H(\vv x_t, \vv m_t) 
& =  -  \dd f(\vv x_t) \tt \dd \phi(\tilde m_t)  +  
 \sup_{d  \in \partial \phi(m_t)} 
 d\tt (\dd f(x_t) - m_t) \\ 
%\dd \phi(\vv m) \tt (\dd f(\vv x_t) - \vv m_t)  \\
& \leq 
\inf_{d \in \partial \phi(m_t)
b \in \partial \phi(\tilde m_t)
} 
\left \{ - \frac{1}{\beta} (\tilde m_t - m_t) \tt (b - d )   - d \tt  \vv m_t \right\} \\
& \leq - \frac{1}{\beta} 
\Delta _\phi(\vv m_t + \beta \dd f(\vv x_t), ~ \vv m_t) - \eta \Delta_\phi (\vv m_t, \vv 0) \leq 0. 
\ee 

%If $\vv m_t =0$, then $\ddtp \lim_{t\to 0^+}\norm{m_{t+u}} - \norm{m_t} =$ then $$\ddt $$

%Define the  right directional derivative of $\phi$ in the direction $d$ as 
 %$$\dd^-\phi(x) = \lim_{\epsilon \to 0^+} \frac{\phi(x+ \epsilon d) - \phi(x)}{\epsilon} $$
 %\red{Proposition 13.2 For any convex function $f\colon\mathbb{R}^n\to (-\infty, \infty]$ and any $\bar x\in{\rm dom}(f)$, the directional derivative $f^\prime(\bar x;d)$ exists for every direction $d\in\mathbb{R}^n$. Furthermore, if $\bar x\in{\rm int}({\rm dom}f)$ then $f^\prime(\bar x;d)$ is a real number for every $d\in\mathbb{R}^n.$}
\url{https://maunamn.wordpress.com/13-directional-derivatives-of-convex-functions/}

\end{proof} 

\begin{lem}
Taking $\phi(x) = \norm{x}_1$, one have  
\bb 
\Delta(x_t,m_t) 
& = \sum_{i=1}^d 2 \ind(\beta g_{t,i} m_{t,i} \leq - m_{t,i}^2) \abs{g_{t,i}}+ \eta \norm{m_t}_1   \\ 
& \geq \sum_{i=1}^d 2 \ind( \abs{g_{t,i} }  \geq \abs{m_{t,i}}/\beta) \abs{g_{t,i}}+ \eta  \norm{m_t}_1  \\
& = 
\ee 
\end{lem}

%Interesting, 

\subsubsection{ 
The interplay of non-smoothness with 
$\beta>0$}
Unlike the smooth (differentiable) case, the counter part result  in Eq \red{xxx} for  $\beta=0$ no longer hold. 
In fact, taking $\phi(x) = \norm{x}_1$ and $\dd\phi(x) = \sign(x)$ and $\beta=0$, and considering the point 
%we have at the point 
$m_t=0$, we have 
$$
\ddtp H(x_t,m_t) =   \sup_{d\in \partial \phi(0)} d \tt \dd f(x_t)  
= \norm{\dd f(x_t)}_1 >0. 
$$



To fix this, we would have to use a better subgradient than $\sign(x)$: 

\begin{thm}
\red{Assume $\alpha>0$ and $\beta=0$}, 
$f$ is differentiable, and 
 $\phi$ is convex on $\RR^d$ 
\red{with $0$ as a minimum point}, 
%whose% unique minimum is $x=0$,  
and denote by $\dd \phi(x)$  the most $f$-ascending subgradient of $\phi$ in that 
$$
\dd^{\uparrow f} \phi(x) \defeq  \argmax_{d \in \partial \phi (x)} \dd f(x) \tt d.   
$$
Then following $\dot x_t = \dd^{\uparrow f} \phi(m_t)$ and $\dot m_t = \dd f(x_t) - \red{\eta} m_t$, we have 
%in that  $\dd \phi(x) \in \partial \phi(x)$ for every $x$. 
%Assume $\red{\alpha, \beta} >0$. 
%Assume $f$ 
 %is differentiable. 
%and $\phi$ is convex with $\vv  0$ as 
%its minimum point.  
%with $\dd\phi(\vv 0)=\vv 0$. 
%Then following \eqref{equ:lionode}, 
%the Hamiltonian $H(\vv x,\vv m)$ decreases monotonically in that 
%in is reviewed a%
$$
\ddtp  H(\vv x_t, \vv m_t)
= 
- \eta D_\phi(\vv m_t, \vv 0) \leq 0, 
$$ 
\end{thm}
\begin{exa}
For $\phi(x) = \norm{x}_1$, we have  
$\dd^{\uparrow f}\phi(x) = [\dd_{x_i}^{\uparrow f}\phi(x)]_{i=1}^d $ with 
\bb 
\dd_{x_i}^{\uparrow f}\phi(x) =  \begin{cases}
\sign(x_i) & \text{if $x_i \neq 0$} \\
\sign(\nabla_{x_i} f(x)) & \text{if $x_i = 0$}.
\end{cases} 
\ee 
One may think 
$\dd_{x_i}^{\uparrow f}\phi(x)
\approx \sign(x + \beta \dd f(x))$ for $\beta \approx 0$. This reveals an intriguing role of having $\beta>0$ in regularizing the system. 
\end{exa}


%1) For hamiltonian system, when $\beta=0$, 
%we should take $\dot x_t = -\dd^f\phi(m)$, 
%where $\dd^f\phi(m)$ is the subgradient of $\phi$ that maximizes its inner product with $\dd f$. 
%2) When $\beta > 0$, 




\section{Derivation of the Mirror Descent Component}

\begin{lem}
Let $h\colon \RR^d\to \RR$ be convex with $0$ with $h(0) =0$ and $\dd h(0) = 0$. 
Let $h^*(y) = \sup_{z} (z \tt y - h(z))$ be the conjugate function of $h$. 

1) $h^*(0)$ and $\dd h^*(0) =0.$

2) For $\alpha >0$ and $\beta \in \RR$, 
the conjugate function of $\tilde h(x) \defeq \alpha  h(\beta x)$ is  $\tilde h^*(x) = \alpha h\left (\frac{x}{\alpha \beta }\right )$. 
\end{lem} 
\begin{proof}
1) Note that $\dd h^*(\dd h(x)) = x$. Taking $x=0$ yields $\dd h^*(0) =0$.
Also, 
$h^*(0) = \sup_{z} (z \tt 0 - h(z)) =   - \inf_z h(z) = h(0)=0$. 

2) 
\bb 
\tilde h^*(x)
& = \sup_{z} \left \{ x\tt z
- \alpha  h(\beta z) \right \}\\ 
& = \sup_{\tilde z}  \alpha \left \{\frac{x}{\alpha  \beta }\tt \tilde z
-   h( \tilde  z) \right \} \ant{$\tilde z = \beta z$}\\ 
& = \alpha h^*\left (\frac{x}{\alpha\beta} \right ). 
\ee 
\end{proof}

\begin{lem} Assume $\phi\colon \RR^d\to\RR$ is convex and $\phi^*$ is its conjugate. 
Let 
\bb 
h_t([x, m])
& =\frac{1}{\beta}
\left ( \phi(m_t + \beta x) -  \phi(m_t)  - \dd  \phi(m_t)\beta  x    \right )+  \red{\eta} \phi^*(\red{\alpha } g_m). 
\ee 
Then the conjugate of $h_t$ is 
$$
h^*_t([y,n]) = \frac{1}{\beta} B_{\phi^*}(y+\dd\phi(m_t), \dd\phi(m_t)) +  \red{\eta }\phi(\frac{n}{\alpha \red{\eta}}).
%B_\phi(n, 0). 
$$
\end{lem}
\begin{proof} 
\bb 
h_t^*([y, n])
& = \sup_{x,m}  \left \{ 
x\tt y + m \tt n - 
\frac{1}{\beta}
\left ( \phi(m_t + \beta x) -  \phi(m_t)  - \dd  \phi(m_t)\beta  x    \right ) -  \eta \phi^*(\alpha m)  \right\} \\ 
& = \sup_{x,m}  \left \{ 
x\tt y  - 
\frac{1}{\beta}
\left ( \phi(m_t + \beta x)  - \dd  \phi(m_t)\tt \beta  x    \right ) \right\} + \frac{1}{\beta} \phi(m_t)  +  \red{\eta }\phi(\frac{n}{\alpha \red{\eta}}) \\
& = \frac{1}{\beta} \left ( \sup_{z,m}  \left \{ 
\left (  (z-m_t) \right) \tt y - 
\left ( \phi(z)   - \dd  \phi(m_t)\tt   (z - m_t)    \right ) \right\} +  \phi(m_t) \right ) 
 + \red{\eta }\phi(\frac{n}{\alpha \red{\eta}})\\
& = \frac{1}{\beta} 
\left ( \sup_{z,m}  \left \{ 
  z  \tt (y+  \dd \phi(m_t)) - 
 \phi(z)    \right\} 
-   m_t\tt y  - \dd\phi(m_t)\tt m_t 
+  \phi(m_t) \right)  +  \red{\eta }\phi(\frac{n}{\alpha \red{\eta}})  \\
& = \frac{1}{\beta} \left ( \phi^*(y + \dd\phi(m_t)) 
-   m_t\tt y  -  \phi^*(\dd\phi(m_t)) \right )  + \red{\eta } \phi(\frac{n}{\alpha \red{\eta}}) \\
& = \frac{1}{\beta} B_{\phi^*}(y+\dd\phi(m_t), \dd\phi(m_t)) +  \red{\eta }\phi(\frac{n}{\alpha \red{\eta}})
\ee 
\end{proof}
